# Supplementary material for: A Novel Algorithm for Rate/Power Allocation in OFDM-based Cognitive Radio Systems with Statistical Interference Constraints
Source: arXiv:1801.07566 source file (2019-02-08)
Supplement: Supplementary file 1 [file appendix_A.tex]

\section*{Appendix A\\Proof of the Optimality of ($\mathbf{b}_m^*,\mathbf{p}_m^*$)}
\vspace{-7pt}
The KKT conditions are written as \cite{Boyd2004convex}
\setlength{\arraycolsep}{0.0em}
\begin{subequations}
\label{eq:KKT}
\begin{IEEEeqnarray}{rCl}
\frac{\partial \mathcal{F}}{\partial \mathcal{P}_{i_m}} + \sum_{\varrho = 1}^{N_m + 2}\lambda_{\varrho} \: \frac{\partial g_\varrho}{\partial \mathcal{P}_{i_m}} &{} = {}& 0, \label{eq:KH1}\\
\frac{\partial \mathcal{F}}{\partial b_{i_m}} +  \sum_{\varrho = 1}^{N_m + 2}\lambda_\varrho \: \frac{\partial g_\varrho}{\partial b_{i_m}} &{} = {}& 0, \label{eq:KH2}\\
g_\varrho \lambda_\varrho &{}={}& 0, \label{eq:KH4} \\
g_\varrho &{} \leq {}& 0, \label{eq:KH5} \\
\lambda_\varrho &{} \geq {}& 0, \label{eq:KH3}
\end{IEEEeqnarray}
\end{subequations}
$i_m = 1, ..., N_m$ and $\varrho = 1, ..., N_m + 2$. One can show that these conditions are satisfied, as sketched in the proof below.
\begin{itemize}
  \item \textit{Proof of} (\ref{eq:KH1}) and (\ref{eq:KH2}): one can find that (\ref{eq:KH1}) and (\ref{eq:KH2}) are satisfied from (\ref{eq:eq1}) and (\ref{eq:eq2}), respectively.
  \item \textit{Proof of} (\ref{eq:KH4}):
  \begin{enumerate}
    \item In all \emph{cases 5 --- 8}, $\mathcal{Y}_{i_m} = 0$; hence from (\ref{eq:slack}),  $g_{i_m}$ is always active, i.e., $g_{i_m} = 0$.
    \item In \emph{case 5}: $\lambda_{N_m+1} = \lambda_{N_m+2} = 0$; hence, $g_{N_m+1} \lambda_{N_m+1} = g_{N_m+2} \lambda_{N_m+2} = 0$.
    \item In \emph{case 6}: $\lambda_{N_m + 2}$ = 0; hence, $g_{N_m +2} \lambda_{N_m +2} = 0$ and $\mathcal{Y}_{N_m + 1} = 0$, and $g_{N_m+1} = 0$ from (\ref{eq:slack}).
    \item In \emph{case 7}: $\lambda_{N_m + 1}$ = 0; hence, $g_{N_m +1} \lambda_{N_m +1} = 0$ and $\mathcal{Y}_{N_m + 2} = 0$, and $g_{N_m+2} = 0$ from (\ref{eq:slack}).
    \item In \emph{case 8}: $\mathcal{Y}_{N_m + 1} = \mathcal{Y}_{N_m + 2} = 0$; hence, $g_{N_m+1} = g_{N_m+2} =  0$ from (\ref{eq:slack}).
  \end{enumerate}
  Thus, $g_\varrho \lambda_\varrho = 0 \quad \forall \quad \varrho = 1, ..., N_m+2$; hence, (\ref{eq:KH4}) is always satisfied.
  \item  \textit{Proof of} (\ref{eq:KH5}): adding non-negative slack variables in (\ref{eq:slack}) guarantees that $g_\varrho \leq 0$; hence, (\ref{eq:KH5}) is always satisfied.
  \item \textit{Proof of} (\ref{eq:KH3}): in \emph{case 5} and from (\ref{eq:eq1}), one finds
\setlength{\arraycolsep}{0.0em}
\begin{IEEEeqnarray}{c}
\lambda_{i_m} = \alpha \Bigg[ 0.2 \: \frac{1.6 \: C_{i_m}}{2^{b_{i_m}-1}} \: \textup{exp}\Big(-1.6 \frac{ C_{i_m} P_{i_m}}{2^{b_{i_m}-1}}  \Big)  \Bigg]^{-1},
\end{IEEEeqnarray}
which is positive for all values of $i_m$. Similarly in \emph{cases 6, 7} and \emph{8}, $\lambda_{N_m + 1}$ and $\lambda_{N_m + 2}$ are found to be positive. Hence, (\ref{eq:KH3}) is always satisfied.
\end{itemize}

As can be seen, the KKT conditions are satisfied, and, thus, the solution ($\mathbf{b}_m^*,\mathbf{p}_m^*$) represents a local optimum point. \hfill$\blacksquare$ %\hfill$\square$
\vspace{-5pt}
